# Supplementary material for: Optimization and Generalization Analysis of Transduction through Gradient Boosting and Application to Multi-scale Graph Neural Networks
Source: arXiv:2006.08550 source file (2021-01-06)
Supplement: Supplementary file 1 [file errata.tex]

\section{Errata}

After the submission of the main paper, we have found several errors. 
We fix them in the camera-ready version.

\begin{itemize}
\item Algorithm 1, l.5: for $t=2\ldots T$ do $\longrightarrow$ for $t=2\ldots T+1$ do
\item l.207: $D^{(t)} = 2\sqrt{2}(2\tilde{B}^{(t)})^{L}\prod_{s=1}^{t-1}\tilde{C}^{(s)}$ $\longrightarrow$ $D^{(t)} = 2\sqrt{2}(2\tilde{B}^{(t)})^{L-1}\prod_{s=2}^{t}\tilde{C}^{(s)}$ 
\item l.208: $P^{(t)}:=\prod_{s=1}^{t-1}\tilde{P}^{(s)}$ $\longrightarrow$ $P^{(t)}:=\prod_{s=2}^{t}\tilde{P}^{(s)}$
\item Theorem 2 (5): $\widehat{\mathcal{R}}(\widehat{Y}) \leq \cdots$ $\longrightarrow$ $\mathcal{R}(\widehat{Y}) \leq \cdots$.
\item Proposition 4 (6): $f(\bm{x}W^{(1)} \cdots W^{(t)})$ $\longrightarrow$ $f(\bm{x}W^{(2)} \cdots W^{(t)})$
\item l.253: $\argmax_{g\in \mathcal{G}^{(t)}_{\mathrm{KTA}}} \rho(g(X^{(t)}), Y)$ $\longrightarrow$ $\argmax_{g\in \mathcal{G}^{(t)}_{\mathrm{KTA}}} \rho(g(X^{(t-1)}), Y)$
\end{itemize}
